# Supplementary material for: A Girl Has A Name: Detecting Authorship Obfuscation
Source: arXiv:2005.00702 source file (2020-05-02)
Supplement: Supplementary file 1 [file appendix.tex]

\section{Appendix}

\begin{figure}
  \centering
  \includegraphics[width=\linewidth]{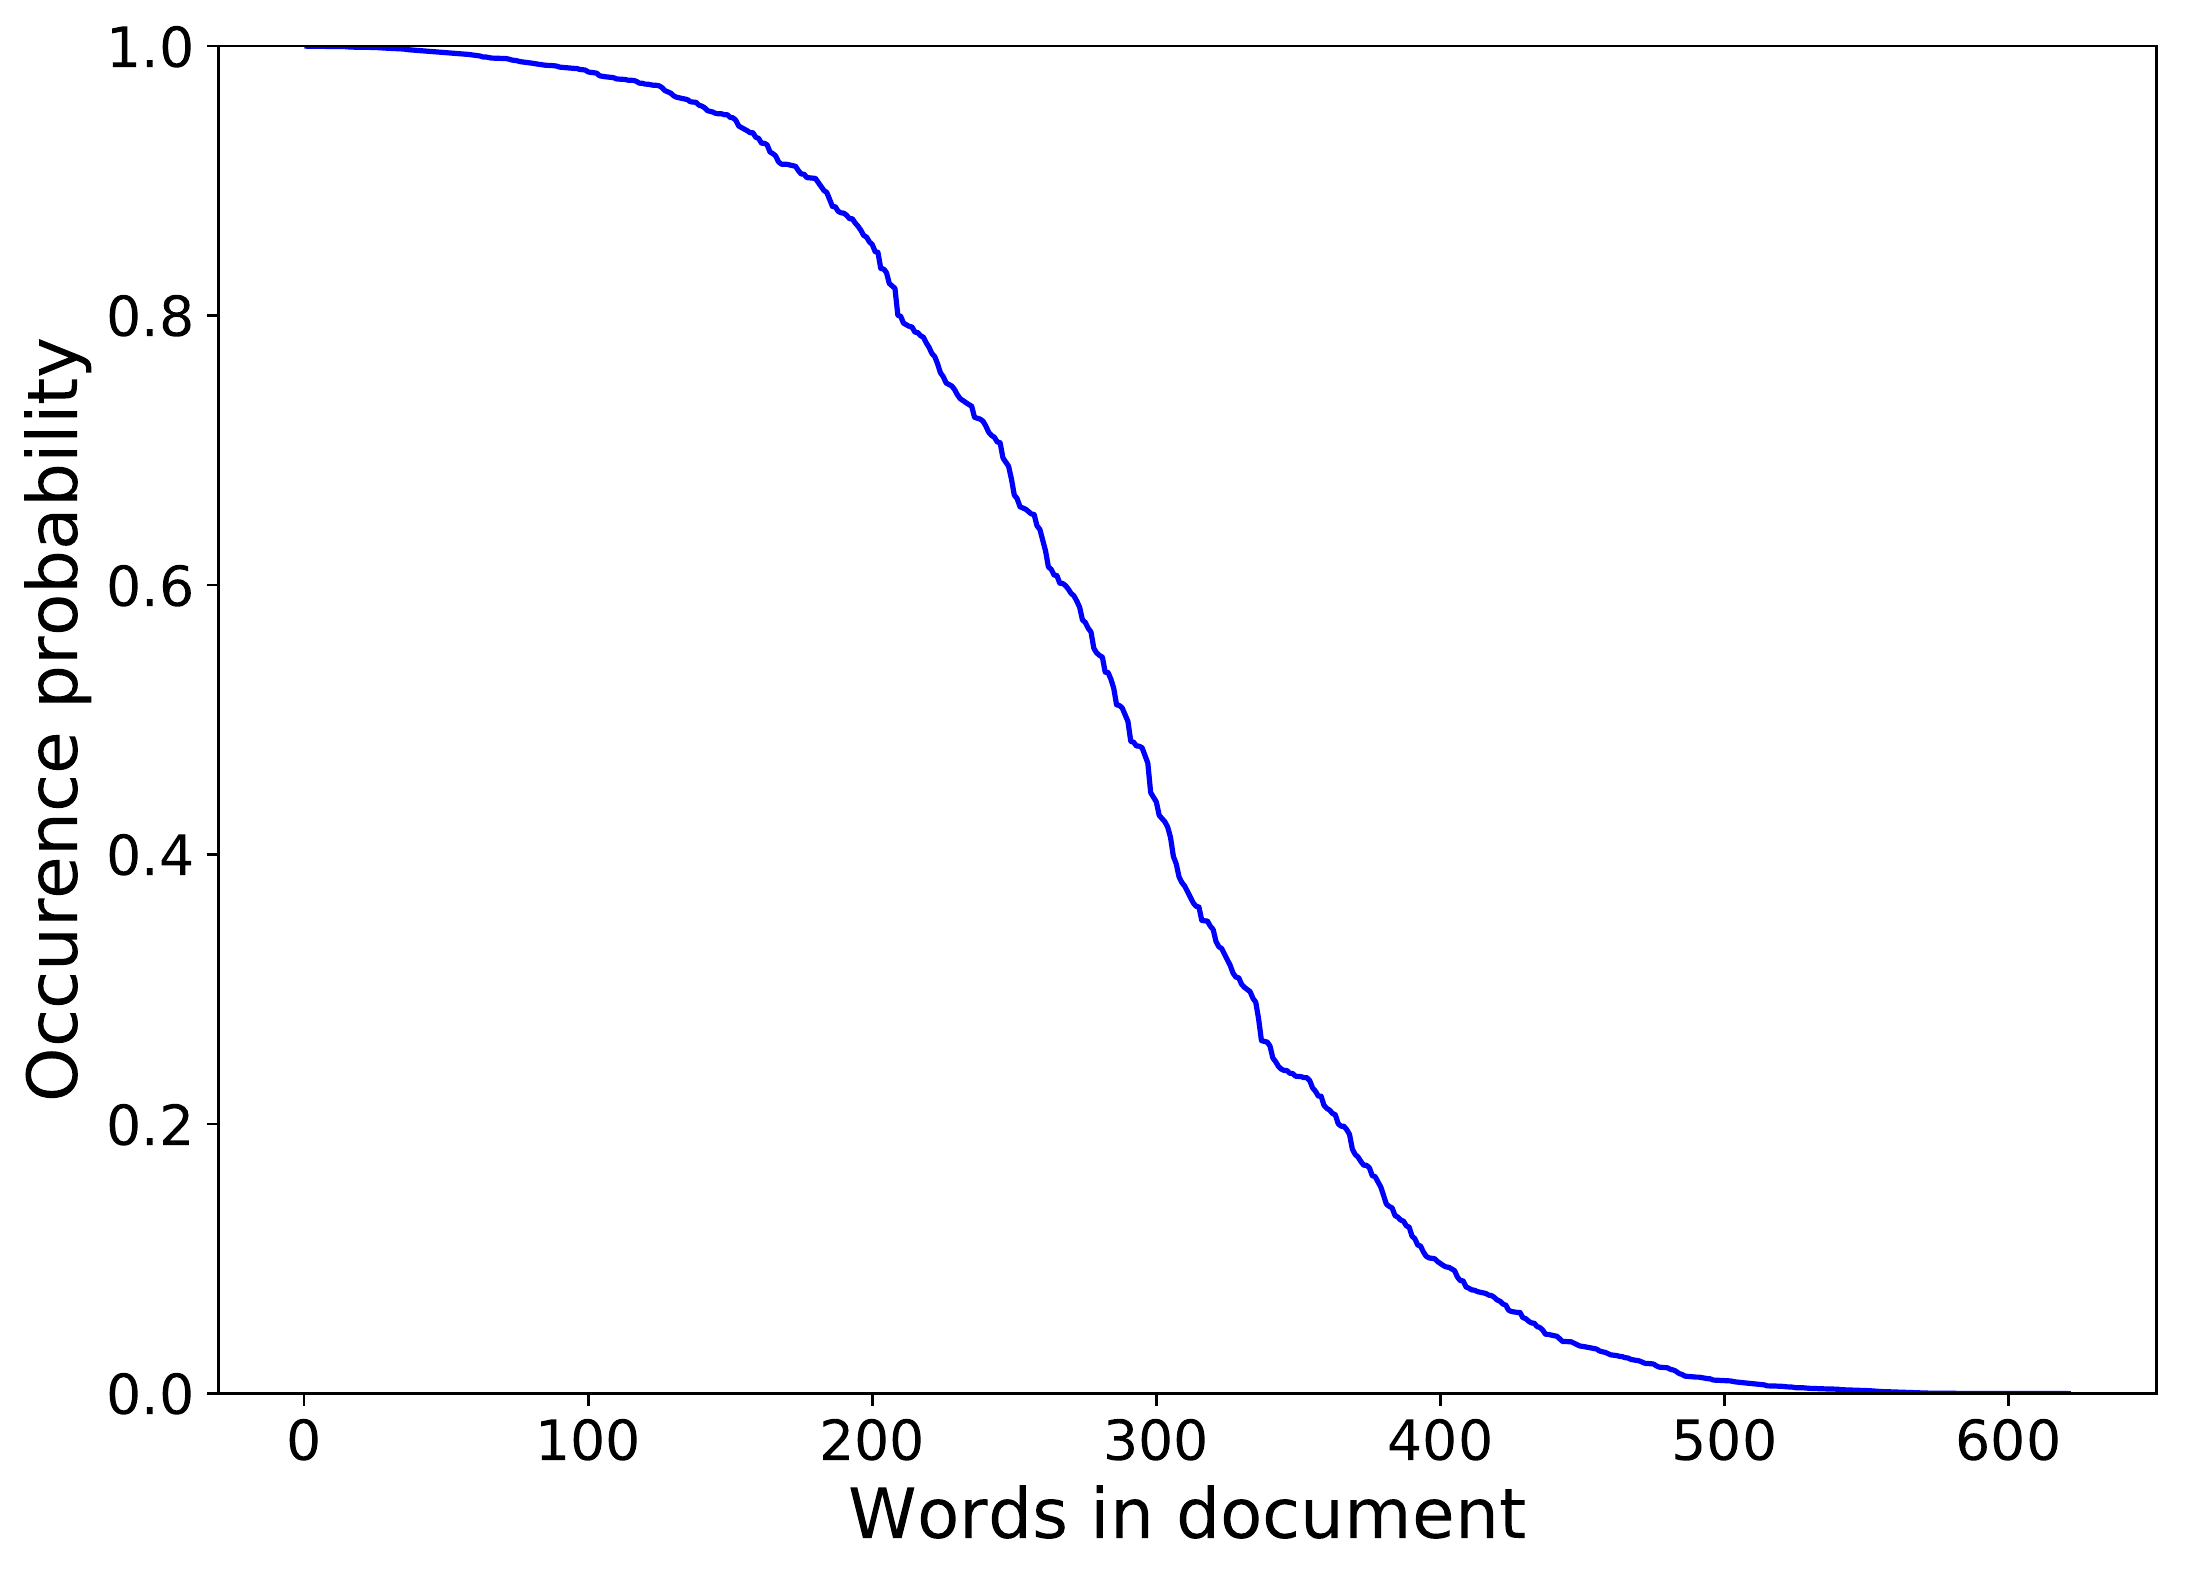}
  \caption{Plot of sorted occurrence probabilities (using \bertsmall model) for a human generated document.}\label{sorted_probs_plot}
\end{figure}
